# Supplementary material for: Distribution through Repeated Market with Buying Rights
Source: arXiv:2505.17271 source file (2025-05-22)
Supplement: Supplementary file 1 [file 01_proofs.tex]

\section{Proofs}
\label{app: proofs}

\begin{cmr}{Theorem \ref{thm:greedy:equilibrial}}
The Greedy strategies given in Eq. \eqref{eq: seller policy} and \eqref{eq: buyer policy} form an equilibrium of a Crisis of any length. 
Furthermore, the equilibrium is coalition-proof and can be computed in polynomial time in the number of buyers and sellers.
\end{cmr}

\input{appendix/01_proof_equilibrium}

\begin{cmr}{Proposition \ref{thm:nonmyo:main}}
Let all traders follow the Greedy strategy. Then the mapping of the current price to the next one is a non-expansive mapping on $\mathbb{R}$ with the L1 norm, resulting in the limiting price being one.
\end{cmr}

\input{appendix/01_proof_nonexpansive}

\begin{cmr}{Theorem \ref{thm:nonmyopic:poa}}
Consider a Crisis where traders follow the Greedy strategy. Then the expected frustration in the Market with the right distribution mechanism is at most $1/2$ of the free market's expected frustration as $\tau \to \infty$.
\end{cmr}

\input{appendix/01_proof_limit_price}

% ================================================

\endinput
\todo[inline]{(D) Tahle část byla v hlavním textu, tady asi nemá co dělat. Navíc odtud dál jsou proof sketche, který taky patří do hlavního textu.}

We start the discussion by showing that, in equilibrium, the price of Good and Right is the same, i.e $p^\tau = q^\tau$. After fixing the prices, we show that no other deviation can benefit any trader.

%Strategic behaviour of the poor buyers is to extract all useless Money from the rich buyers in the second market mechanism stage by selling Right, which can be used to fix $q^\tau$ after $p^\tau$ is known. What remains is to fix the price of Good $p^\tau$. 
Seemingly, the sellers can simply choose the (free) market-clearing price 
$p^\tau = \frac{\sum_{b\in B} M^\tau_b}{\sum_{b\in B} R^\tau_b} = \frac{\sum_{b\in B} M^\tau_b}{\sum_{s\in S} G^\tau_s}$, which would imply 
$\sum_{b\in B} M^\tau_b = \Delta M_S^\tau \Rightarrow \Delta M_B = 0 \Rightarrow q^\tau = 0$. However, a poor buyer would not sell the Right for free, since increasing the price gives him more Money for the next Market, increasing his utility\footnote{Furthermore, decreasing the amount of Good sold would decrease the price in the following Market.}. This would imply that not all Good would be sold, decreasing the sellers' utility. Therefore $p^\tau < \frac{\sum_{b\in B} M^\tau_b}{\sum_{b\in B} R^\tau_b}$, leaving some $\Delta M_B > 0$ which the poor buyers split among themselves. 

In fact, the sellers want to set the price very precisely.
\begin{lemma}\label{thm: equal prices}
Let $p^\tau$ and $q^\tau$ be the selling price of Good and Right, declared by all sellers and buyers, respectively. Then it is not profitable for any trader to deviate if and only if $p^\tau = q^\tau$.
\end{lemma}

\begin{sproof}
If $p^\tau > q^\tau$, then buyers can sell Right at higher price, increasing their utility. If $p^\tau < q^\tau$, then all seller can increase the price, resulting in higher utility for them.
\end{sproof}

With this results, we can now outline the main idea discussed in the rest of this Section. Any deviation by any trader from SOMETHING will either have no effect on the Market, or will result in less Good being sold. The main idea is in how the price will change in the following Market. We will denote all variables in this alternative scenario with a hat; note that $\hat{p}^\tau = p^\tau$, $\hat{M}_b^\tau = M_b^\tau$, $G^\tau_s=\hat{G}^\tau_s$, and $\hat{R}_b^\tau \le R_b^\tau$.

Let us begin the discussion with the sellers. Let $s$ deviate and offers less Good $v_s^\tau = g_s - {\cal V}$ in hope that the price in SOMETHING goes up in the following Markets. It turns out the seller would be better of just following SOMETHING.

\begin{lemma}\label{lm:nonmyo:utildec}
Let a seller $s$ offer less Good in $\tau$, and sell it in the following Market. Then his utility decreases as a consequence.
\end{lemma}
\begin{sproof}
Comparing the situations in which $s$ offers everything and keep something for the next Market, we get the price in the latter scenario is weighted average of the current and former prices. So either the price goes up, and it would have been beneficial to sell in the next Market, or it goes down, in which case selling in the current Market is better.
\end{sproof}

%Using Eq. (\ref{eq: next money}) thus implies $\hat{M}_b^{\tau+1} \le M_b^{\tau+1}$. As we showed in the proof of Lemma \ref{lemma: next price}, the price is an increasing function of the Money\footnote{This was derived for the same volume being offered in both Markets. Here, since in the next Market the volume is larger, the price will decrease even more. This is assuming $s$ deviates in the following Market as well and offers $g_s + {\cal V}$. If he doesn't he loses even more utility.}, so we also have $\hat{p}^{\tau+1} \le p^{\tau+1}$.\todo{(D) This part is likely wrong, needs more work.}

It remains to show that similar strategy is not advantageous for a buyer. Similar reasoning we used for the seller suggest that the price should decrease, but it is not the case. This is because, following SOMETHING, the sellers will offer the same volume of Good, leading to the same distribution of Right as in the last Market. Also, since some Good wasn't sold, $\sum_{b\in B}\hat{M}^{\tau+1}_b = \sum_{b\in B}M^{\tau+1}_b + p^\tau {\cal V}$, so $\hat{p}^{\tau+1} > p^{\tau+1}$. Moreover, if $b$ was poor in $\tau$, then he will receive less Money from selling Right, limiting the amount of Good he can buy in the next Market
\begin{equation*}
    \hat{M}^{\tau+1}_b = m_b + \max\{0, p^{\tau} (R_b-{\cal V}) - M^{\tau}_b\} < M^{\tau+1}_b.
\end{equation*}
\todo[inline]{(D) This might also be formulated as a Lemma so that it could be used in the following Theorem.}

Consider now a deviation in the last Market of the Sequence. Clearly, if less Good is sold, then no trader can gain utility. It is thus not beneficial to deviate in the last Market of the Sequence from SOMETHING.
Above we showed that deviating and following SOMETHING in the following Market is not beneficial for any trader, so they are incentivised to follow SOMETHING in the second-last Market. Inductive reasoning leads to the following Theorem.\todo[inline]{(D) Since the traders are Markovian, does this really make sense? They cannot choose to deviate in the second last Market. But this should be sufficient to show that no Markovian trader wants to deviate either.}
